# Supplementary material for: One-dimensional magnetic order in the metal-organic framework Tb(HCOO)3
Source: arXiv:1605.02575 source file (2016-05-09)
Supplement: Supplementary file 1 [file 2016_tbformate_si.pdf]

# One-dimensional magnetic order in the metal-organic framework $Tb(HCOO)_3$

# Supplementary Information

Daniel R. Harcombe,[1] Philip G. Welch,[1,2] Pascal Manuel,[2]
Paul J. Saines,[3*] and Andrew L. Goodwin[1]

6th May 2016

[1]Department of Chemistry, University of Oxford, Inorganic Chemistry Laboratory,
South Parks Road, Oxford OX1 3QR, U.K.
[2]ISIS Facility, Rutherford Appleton Laboratory, Chilton, Didcot,
Oxfordshire OX11 0QX, U.K.
[3]School of Physical Sciences, University of Kent, Canterbury, CT2 7NH, U.K.
[*]Electronic address: P.Saines@kent.ac.uk

# Contents

**S1 Rietveld Refinement Details** **3**

**S2 SPINVERT Refinements with Ising Degrees of Freedom** **5**

**S3 DMC Parameter Grid Search** **6**

**S4 Analysis of Single-Ion Anisotropy and Spin Correlation Functions** **10**

**S5 Generation of Large Supercell for Total Scattering Calculation** **12**

**S6 References** **13**

## S1 Rietveld Refinement Details

The nuclear and magnetic structures of $Tb(HCOO)_3$ were refined against the neutron scattering data collected at 1.6 K using the GSAS software [S7]. Basic crystallographic details are given in Table S1 and the refined atom positions and magnetic moments are listed in Table S2. Note that in the magnetic space group $P3m'1$, the Tb moments are constrained to lie along **c**. An illustration of the Rietveld fit obtained is given in Fig. S1. Use of the same profile parameters for both nuclear and magnetic Bragg reflections revealed a small additional broadening to the magnetic component, as is evident in the residual function for the highest $d$-spacing reflections shown in Fig. S1. The magnetic model used for these refinements is that proposed by Kurbakov et al. [S3]

**Table S1:** Crystallographic details determined by time of flight neutron powder diffraction.

| | |
|---|---|
| Empirical formula | $TbC_3D_3O_6$ |
| Formula weight ($g\,mol^{-1}$) | 296.957 |
| Crystal system | Rhombohedral |
| Nuclear space group | $R3m$ (No. 160) |
| Magnetic space group | $P3m'1$ (translationgleiche; Fedorov space group No. 156) |
| Radiation | neutron, time of flight |
| Temperature (K) | 1.6 |
| $a$ (Å) | 10.42047(12) |
| $c$ (Å) | 3.96889(5) |
| Number of observations | 15 569 |
| $R_p$ | 0.0459 |
| $wR_p$ | 0.0452 |
| $\chi^2$ | 53.91 |

**Table S2:** Refined structural model determined using time-of-flight powder neutron diffraction. *This coordinate was fixed, as required in the polar space group $R3m$.

| Atom | Wyckoff site | $x$ | $y$ | $z$ | $U_{\text{iso}}$ (Å$^2$) | moment ($\mu_{\text{B}}$) |
|---|---|---|---|---|---|---|
| Tb | $3a$ | 0 | 0 | 0* | 0.0121(5) | −2.351(17) / 1.176(8) |
| C | $9b$ | 0.51342(7) | 0.48658(7) | 0.2167(5) | 0.0107(3) | – |
| O1 | $9b$ | 0.46669(7) | 0.53331(7) | −0.0130(5) | 0.0103(3) | – |
| O2 | $9b$ | 0.58314(6) | 0.41686(6) | 0.1715(6) | 0.0099(3) | – |
| D | $9b$ | 0.49501(7) | 0.50499(7) | 0.4778(5) | 0.0267(5) | – |

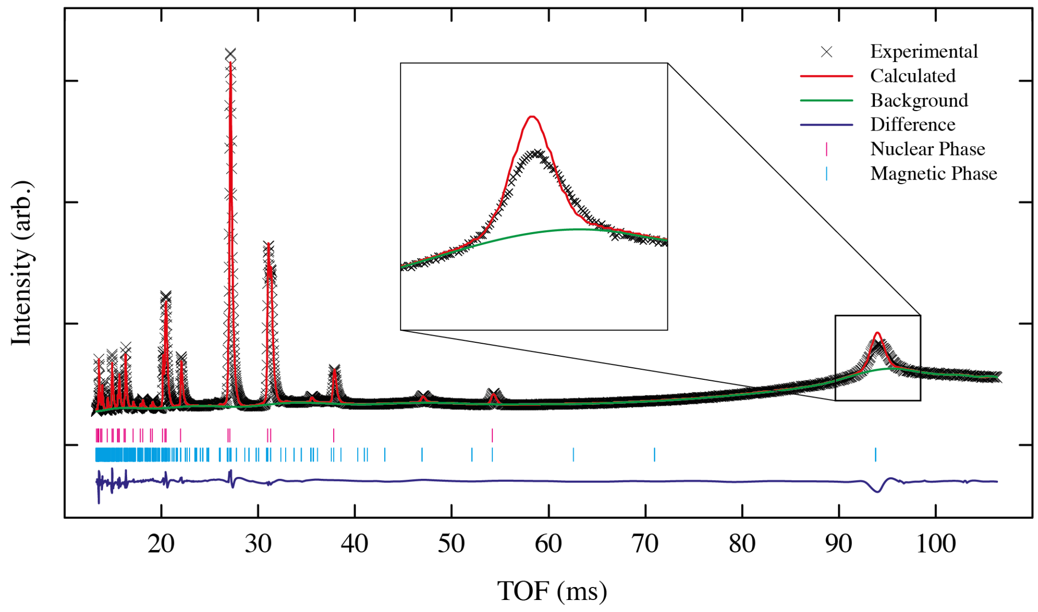


**Figure S1:** Rietveld fit to neutron diffraction data measured at 1.6 K for the $Tb(DCOO)_3$ structural parameters given in Tables S1 and S2. Inset is a larger representation of the low-Q magnetic peak

## S2 SPINVERT Refinements with Ising Degrees of Freedom

In order to provide an upper bound on the degree of single-ion anisotropy consistent with our neutron scattering measurements, we carried out a parallel series of SPINVERT refinements where $Tb^{3+}$ spins were treated as Ising variables. In all other respects the refinements followed the same protocols (configuration size, equilibration, *etc.*) as for the Heisenberg refinements described in the main text. The fits obtained are shown in Fig. S2, from which it is clear that the only significant differences are found at lowest-$Q$. We conclude that the neutron scattering data are consistent with strong easy-axis anisotropy, although clearly do not require absolute anisotropy given the quality of fits shown in Fig. 2(a) of the main text.

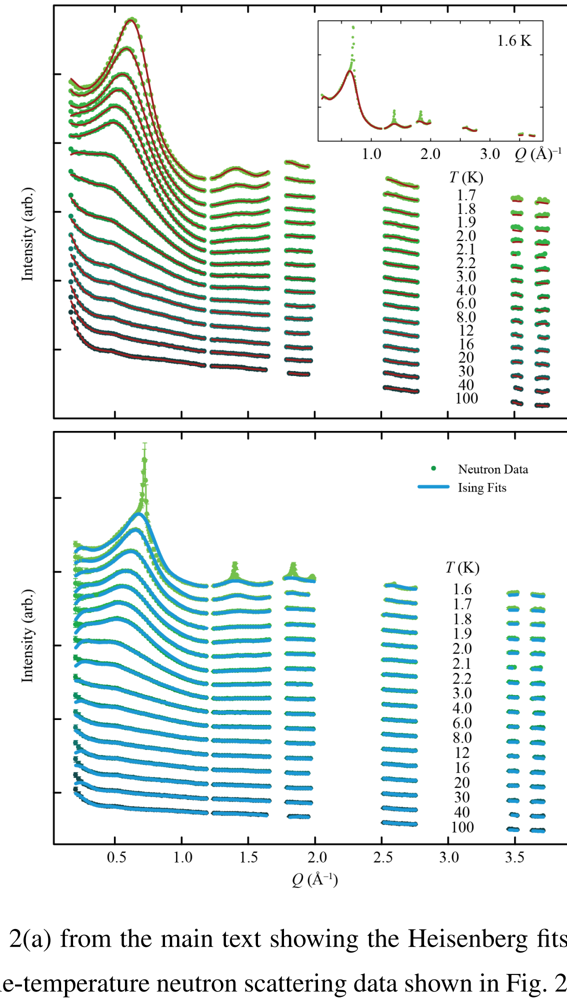


**Figure S2:** Top Pane is Fig. 2(a) from the main text showing the Heisenberg fits. Bottom pane shows the Ising SPINVERT fits to the variable-temperature neutron scattering data shown in Fig. 2 of the main text. Here, data are shown as solid symbols and fits as blue lines. The experimental uncertainty is included as vertical error bars.

## S3 DMC Parameter Grid Search

In order to identify a suitable set of parameters $J_{\|}, J_{\perp}, D$ for the simple Hamiltonian proposed in the main text (Eq. (2) of the main text), we used DMC simulation driven by that Hamiltonian for a range of $J_i, D$ values and assessed each simulation according to its ability to reproduce the pairwise spin correlation functions obtained from our SPINVERT refinements. Independent DMC simulations were performed 20 times for each parameter set; the simulation temperature was cooled from 100 K to 1.7 K, allowing for equilibration at each temperature point (monitored using the autocorrelation functions). For selected parameter sets we ran additional checks by carrying out 100 independent simulations; we found less than $1\%$ variation in residual values in these cases. Because of the extremely large parameter space to be explored, we focussed on carefully-chosen cuts through parameter space in order to most easily identify the optimal parameter sets. The results of this grid search are represented graphically in Fig. S3. The very best fits are obtained for large values of $D$, and the optimal parameter set is that descried in the main text. The corresponding reproduction of the spin correlation functions is shown in Fig. S4.

There is clearly a range of $D$ values for which acceptable reproductions of the pairwise spin correlation functions can be obtained. We do not attach too great a significance to the absolute values of $J_{\|}, J_{\perp}, D$ we report, since our interest is primarily in the intermediate order state that emerges at 1.6 K. We actually find that all reasonable parameter sets result in a transition to the same partially ordered state in DMC simulations. We illustrate this point by showing in Fig. S5 representations of the ordered state obtained for two different parameter sets. Additional experimental measurements may help constrain more accurately the $J_i, D$ values, and exploration of a more complex Hamiltonian that distinguishes $J_2$ and $J_3$ exchange pathways (see Fig. 1(b) of the main text) may provide an even more faithful reproduction of the experimental spin correlation functions. Neither additional measurement nor additional interaction complexity, however, is required to identify the basic nature of the intermediate order state in $Tb(HCOO)_3$.

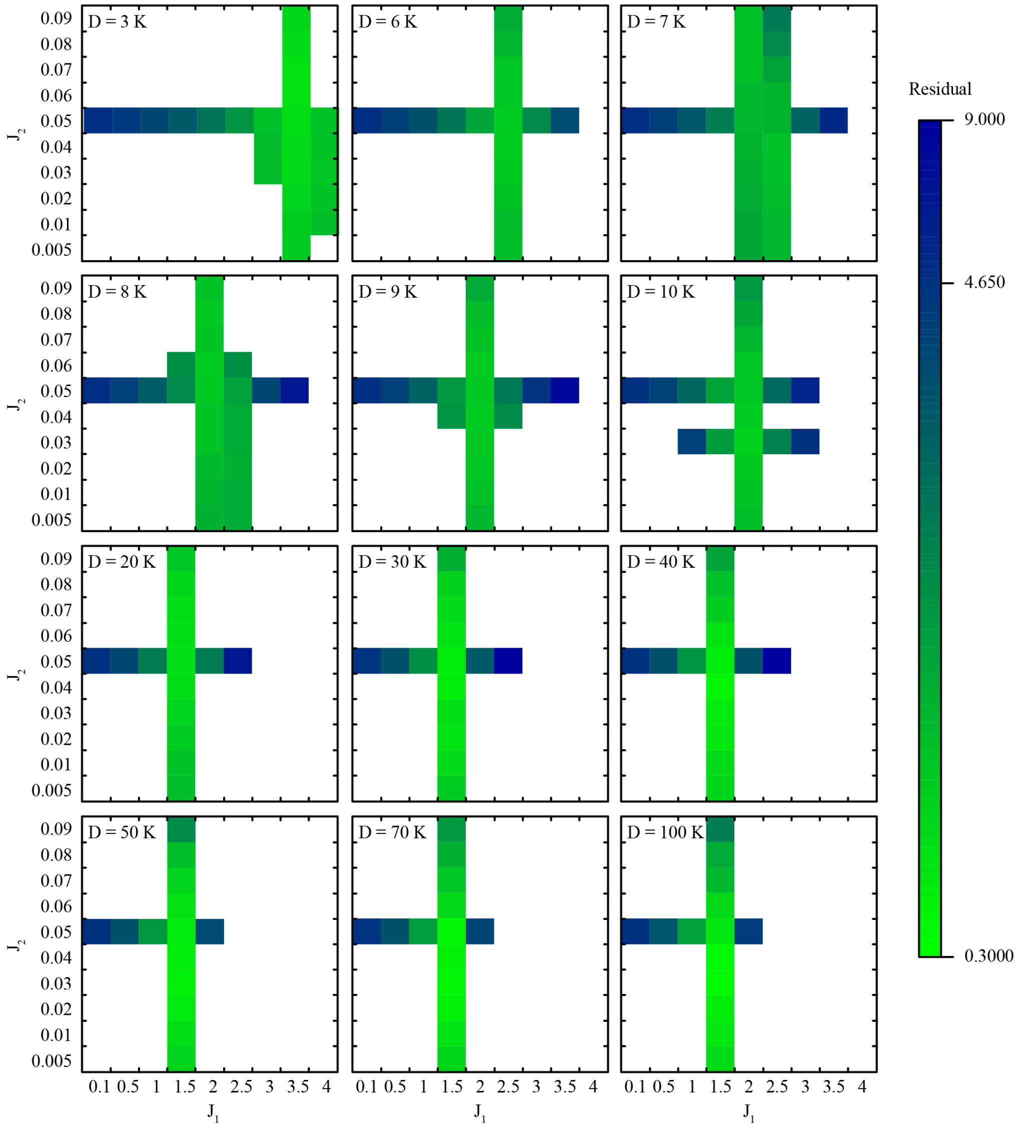


**Figure S3:** Graphical representation of the DMC parameter grid search used to determine the values of $J_{\parallel} = J_1$, $J_{\perp} = J_2$, and $D$ reported in the main text. The colour of each square quantifies the ability of a set of 20 independent DMC simulations driven by a given parameter set to reproduce the pairwise spin correlation functions extracted from experimental neutron scattering data using SPINVERT refinement.

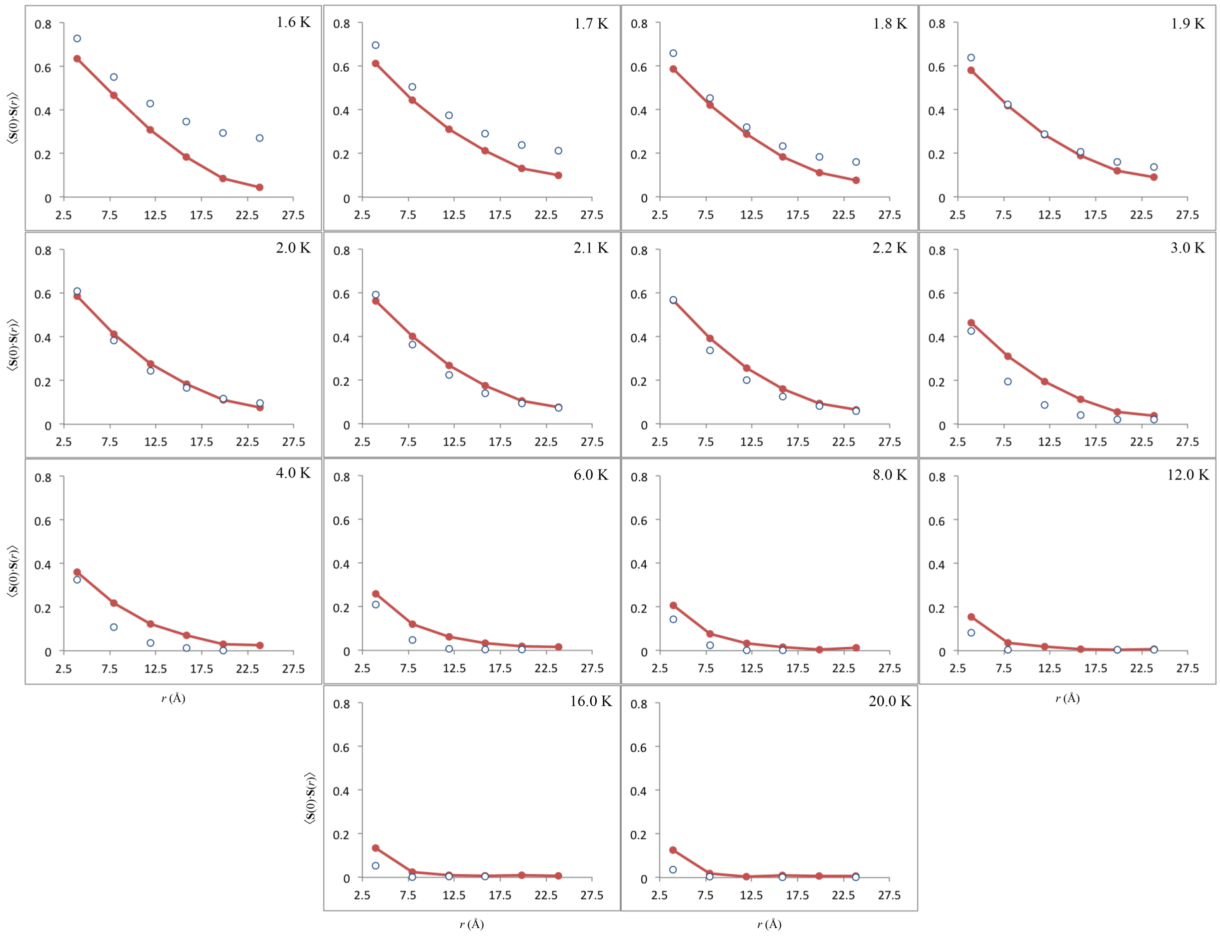


**Figure S4:** Comparison of experimental (SPINVERT) and DMC intra-chain spin correlation functions throughout the paramagnetic regime. SPINVERT results are shown using filled red circles; DMC results are shown as open blue circles. Uncertainties are smaller than the symbols.

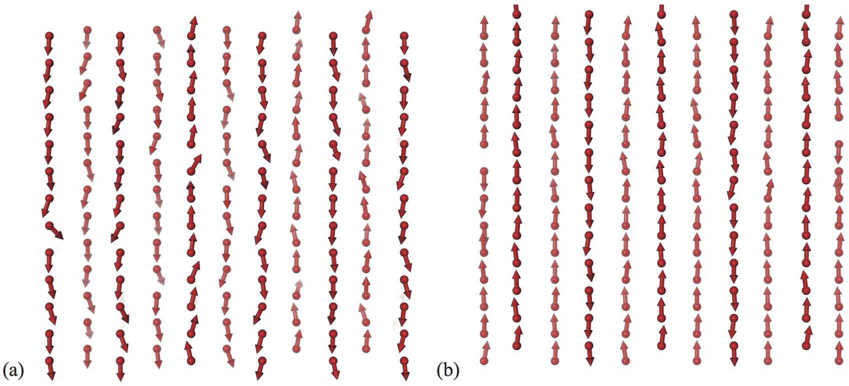


**Figure S5:** Representative sections of 1 K DMC configurations driven using two different parameter sets, each of which is capable of a good description of the paramagnetic spin correlation functions over the temperature range 1.7–100 K: (a) $J_{\|} = 2\,\mathrm{K}$, $J_{\perp} = 0.03\,\mathrm{K}$. $D = 10\,\mathrm{K}$; (b) $J_{\|} = 1.5\,\mathrm{K}$, $J_{\perp} = 0.03\,\mathrm{K}$. $D = 70\,\mathrm{K}$. In both cases the DMC simulations have ordered on cooling below $1.7\,\mathrm{K}$ to give a state equivalent to the TIA state described in the main text.

# S4 Analysis of Single-Ion Anisotropy and Spin Correlation Functions

In this section we present some direct analysis of the single-ion anisotropy and pairwise spin correlation functions determined from our SPINVERT [S1, S2] fits to the neutron scattering data shown in Fig. 2(a) of the main text and also the DMC simulations described in the article. Considering first the extent of single-ion anisotropy—noting that the SPINVERT results represent a lower-bound on the true anisotropy—we use as our measure the ratio of maximum and minimum orientational distribution densities $\Delta \ln(p) = \ln(p_{\rm max}) - \ln(p_{\rm min})$. The temperature dependence of this function is shown in Fig. S6(a) for both SPINVERT refinements and DMC simulations. We find an approximate power-law dependence below 10 K, with vanishing anisotropy at higher temperatures.

We then investigated the intra-chain spin correlation functions, fitting our experimental values using the empirical expression

$$\langle \mathbf{S}(0) \cdot \mathbf{S}(r, T)\rangle = A(T) \exp[-r/\xi(T)]. \tag{S1}$$

Here $\xi$ can be interpreted as a measure of the spin correlation length, and $A < 1$ allows for the population of spin waves ($A \to 1$ in the Ising limit). Our fits to the SPINVERT correlation functions and the corresponding values of the parameters $\xi$, $A$ for both SPINVERT and DMC configurations are shown in Fig. S6(b,c). In the SPINVERT case we again find an approximate power-law dependence for both $\xi$ and $A$ for $T < 10$ K; the fits are not well

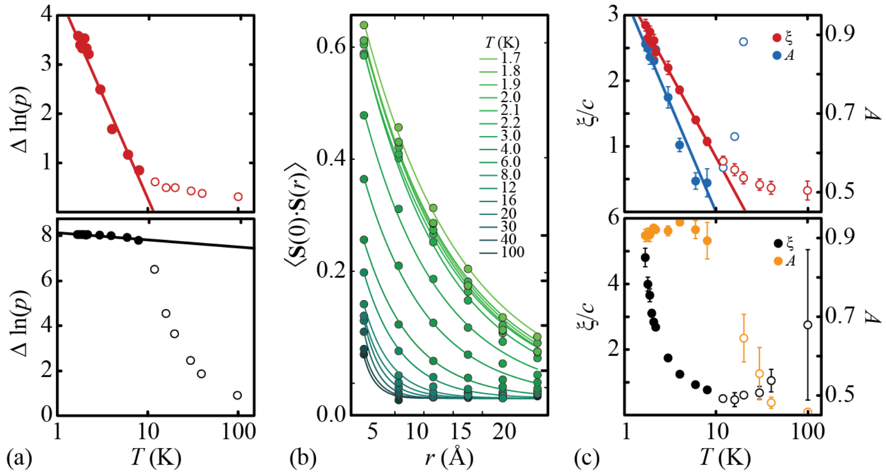


**Figure S6:** Temperature dependence of magnetic order in $Tb(HCOO)_3$. (a) Temperature dependence of the single-ion anisotropy, as determined from the SPINVERT refinements (red symbols; top panel) and DMC simulations (black symbols; bottom panel). (b) Intra-chain spin correlation functions, determined from SPINVERT configurations as described in the text. The solid lines show least-squares fits obtained using Eq. (S1). (c) $T$-dependence of the intra-spin correlation length and prefactor, extracted from the fits shown in (b) (red and blue symbols; top panel) and from analysis of DMC configurations (black and orange symbols; bottom panel). The solid lines show fits to the low-$T$ experimental values (filled symbols) where appropriate.

constrained above 10 K. The Ising formalism $c/\xi = \ln[\coth(J/T)]$ [S4] could not provide a convincing fit to our SPINVERT correlation functions; we interpret this failure of the strict Ising model as an indication of the relevance of the energy scale of $D$ (here evidenced also by the temperature dependence of $A$), which distinguishes this system from systems such as $Ca_3Co_2O_6$ where Ising behaviour is sufficient to fit the experimental spin correlation functions [S5, S6].

# S5 Generation of Large Supercell for Total Scattering Calculation

We briefly describe the generation of the large spin configuration from which the total scattering pattern (*i.e*, including both Bragg and diffuse components) shown in Fig.3(b) of the main text was calculated. First, using a custom Monte Carlo code, we derived a large 2D configuration corresponding to a ground (zero-defect) state of the Ising nearest-neighbour triangular antiferromagnet. The configuration size we used corresponded to a $4 \times 4$ supercell of the $(001)$ projection of the original SPINVERT configuration described in the main text. By assigning the spin of an atom in the 3D supercell to be the same as that of its projection on to the $(001)$ plane, we proceeded to expand this 2D Ising configuration into a 3D Heisenberg spin configuration. This then corresponded to a $4 \times 4 \times 4$ supercell of the original SPINVERT/DMC configuration. In doing so each Ising state $\epsilon$ of the 2D configuration was used to generate the spin vector $\mathbf{S}$ of a column of spins in the 3D configuration:

$$\epsilon \in \{-1, +1\} \rightarrow \mathbf{S} = (0, 0, \epsilon). \tag{S2}$$

The 3D spin configuration was then used as a input for an additional SPINVERT refinement, now allowing small reorientations of the spins; the aim here was to introduce small fluctional movements of the spins as would be permitted at finite temperature. Note that the size of the configuration meant that a full SPINVERT refinement from a random spin arrangement was computationally unfeasible. Instead our aim was simply to show that a sensible spin configuration based on the intermediate ordered state identified in DMC simulations could account for the observed neutron diffraction pattern. After sufficient SPINVERT refinement cycles to allow 25 proposed moves / spin, we obtained a calculated magnetic diffraction pattern that was in good agreement with the experimental data; the resulting configuration is that described in the text and used to generate Fig. 3(b).

## S6 References


[S1] J. A. M. Paddison and A. L. Goodwin, *Phys. Rev. Lett.* **108**, 017204 (2012).

[S2] J. A. M. Paddison, J. R. Stewart, and A. L. Goodwin, *J. Phys.: Cond. Matt.* **25**, 454220 (2013).

[S3] A. I. Kurbakov, J. Rodriguez-Carvajal, V. A. Trounov, and N. V. Starostina, *Mater. Sci. Forum* **321-324**, 971 (2000).

[S4] R. J. Baxter, *Exactly Solved Models in Statistical Mechanics* (Academic, New York, 1982).

[S5] L. Chapon, *Phys. Rev. B* **80**, 172405 (2009).

[S6] J. A. M. Paddison, *et al.*, *Phys. Rev. B* **90**, 014411 (2014).

[S7] R. von Dreele and A. C. Larson, GSAS General Structure Analysis System, Los Alamos National Laboratory Report No. LAUR 86-748, 1986 (unpublished).
